# Supplementary material for: A polarizable CASSCF/MM approach using the interface between OpenMMPol library and CFour
Source: arXiv:2411.12489 source file (2024-11-19)
Supplement: Supplementary file 1 [file suppinfo.pdf]

## Supporting Information for:
## A polarizable CASSCF/MM approach using the interface between OpenMMPol library and CFour

Tommaso Nottoli[1], Mattia Bondanza[1], Filippo Lipparini[1] and Benedetta Mennucci[1]

[1]Dipartimento di Chimica e Chimica Industriale, Università di Pisa, Via G. Moruzzi 13, I-56124 Pisa, Italy

### S1. Additional calculations for Dronpa system

We report in the following tables further results obtained using different active spaces for the CASSCF method. In particular we show in Table S1 the bond length alternation (BLA) parameter, in Table S2 the hydrogen-bond lengths, and in Table S3 the value of the dihedral angle formed by the carbon atoms connecting the benzene moiety to the imidazole ring of Dronpa's chromophore.

**Table S1.** BLA values (in Å) for Dronpa's chromophore computed with different CAS active spaces computed in vacuum and in the protein with the two different force fields.

| Method | Vacuum | Amber | AMOEBA |
|---|---|---|---|
| CAS(4,4) | 0.027 | 0.002 | -0.018 |
| CAS(8,8) | 0.037 | -0.004 | -0.017 |
| CAS(10,10) | 0.048 | -0.004 | -0.020 |
| CAS(12,12) | 0.041 | 0.010 | -0.020 |

**Table S2.** Hydrogen bond lengths between the two oxygen atoms of Dronpa's chromophore and the residues/water. All values are in Å.

| | **Ser** | | **Wat** | | **Arg$_1$** | | **Arg$_2$** | | **Arg$_3$** | |
|---|---|---|---|---|---|---|---|---|---|---|
| **Method** | Amber | AMOEBA | Amber | AMOEBA | Amber | AMOEBA | Amber | AMOEBA | Amber | AMOEBA |
| CAS(4,4) | 1.743 | 1.790 | 1.740 | 1.834 | 1.886 | 1.950 | 2.459 | 2.504 | 1.781 | 1.926 |
| CAS(8,8) | 1.741 | 1.785 | 1.738 | 1.827 | 1.909 | 1.952 | 2.450 | 2.506 | 1.795 | 1.930 |
| CAS(10,10) | 1.740 | 1.788 | 1.736 | 1.830 | 1.909 | 1.969 | 2.449 | 2.509 | 1.795 | 1.951 |
| CAS(12,12) | 1.751 | 1.787 | 1.742 | 1.828 | 1.898 | 1.970 | 2.455 | 2.508 | 1.787 | 1.952 |

**Table S3.** Dihedral angle in degrees for Dronpa's chromophore.

| Method | Vacuum | Amber | AMOEBA |
|---|---|---|---|
| CAS(4,4) | 180 | 175 | 174 |
| CAS(8,8) | 180 | 175 | 174 |
| CAS(10,10) | 180 | 175 | 173 |
| CAS(12,12) | 180 | 174 | 173 |

## S2. Additional calculations for OCP system

Additional data is provided also for the OCP system. In the tables below, we present results obtained using various CAS active spaces for the geometrical parameters investigated in the main paper. Specifically, we report in Table S4 the BLA, in Table S6 the hydrogen-bond lengths, in Table S5 the angle form between the oxygen of CAN and the two residues.

**Table S4.** BLA values (in Å) for OCP's chromophore computed with different CAS active spaces computed in vacuum and in the protein with the two force fields.

| Method | Vacuum | Amber | AMOEBA |
|---|---|---|---|
| CAS(8,8) | 0.157 | 0.149 | 0.152 |
| CAS(8,10) | 0.157 | 0.150 | 0.149 |
| CAS(8,12) | 0.151 | 0.147 | 0.149 |
| CAS(10,12) | 0.141 | 0.143 | 0.142 |
| CAS(12,12) | 0.155 | 0.136 | 0.139 |
| CAS(12,14) | 0.149 | 0.154 | 0.134 |

**Table S5.** Angle between the oxygen atom of CAN and the two residues (Trp-288 and Tyr-201).

| Method | Amber | AMOEBA |
|---|---|---|
| CAS(8,8) | 90 | 87 |
| CAS(8,10) | 90 | 87 |
| CAS(8,12) | 90 | 87 |
| CAS(10,12) | 90 | 87 |
| CAS(12,12) | 90 | 87 |
| CAS(12,14) | 90 | 87 |

**Table S6.** Hydrogen bond lengths. All values are in Å.

| | **Trp-288** | | **Tyr-201** | |
|---|---|---|---|---|
| **Method** | Amber | AMOEBA | Amber | AMOEBA |
| CAS(8,8) | 1.878 | 1.924 | 1.864 | 1.921 |
| CAS(8,10) | 1.878 | 1.925 | 1.864 | 1.924 |
| CAS(8,12) | 1.879 | 1.925 | 1.869 | 1.924 |
| CAS(10,12) | 1.879 | 1.925 | 1.870 | 1.926 |
| CAS(12,12) | 1.881 | 1.928 | 1.876 | 1.932 |
| CAS(12,14) | 1.877 | 1.928 | 1.859 | 1.934 |
